# Supplementary material for: EBS-EKF: Accurate and High Frequency Event-based Star Tracking
Source: arXiv:2503.20101 source file (2025-03-25)

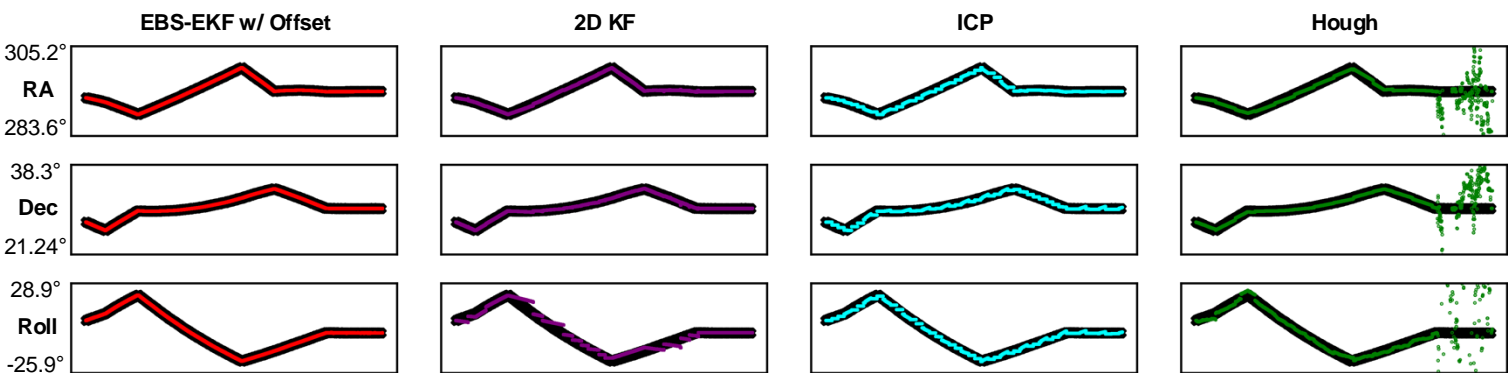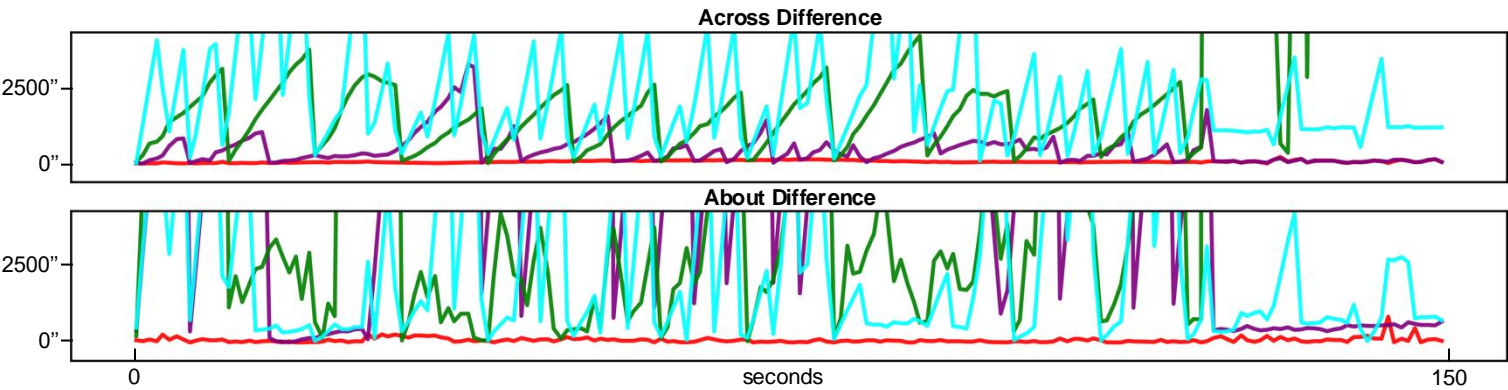

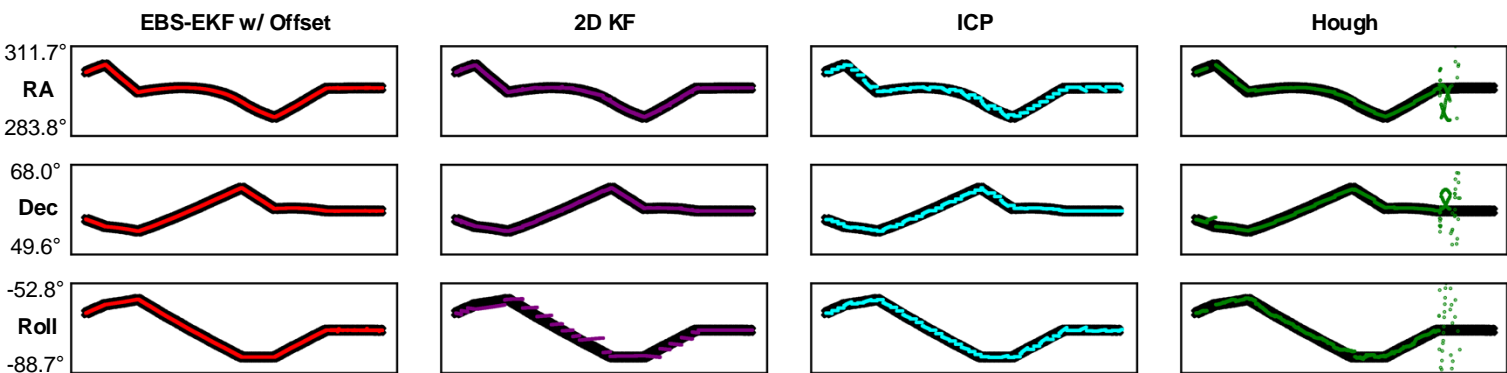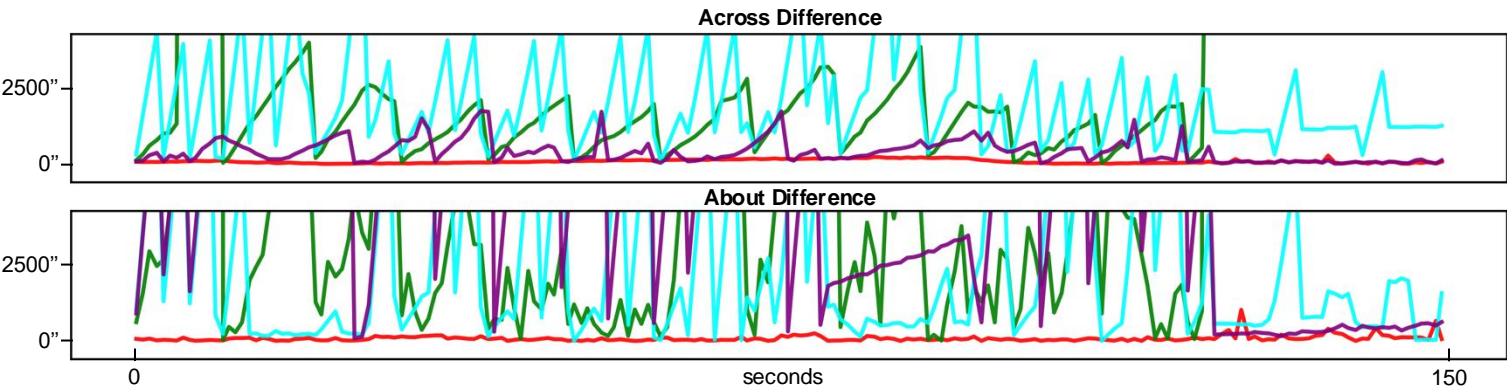

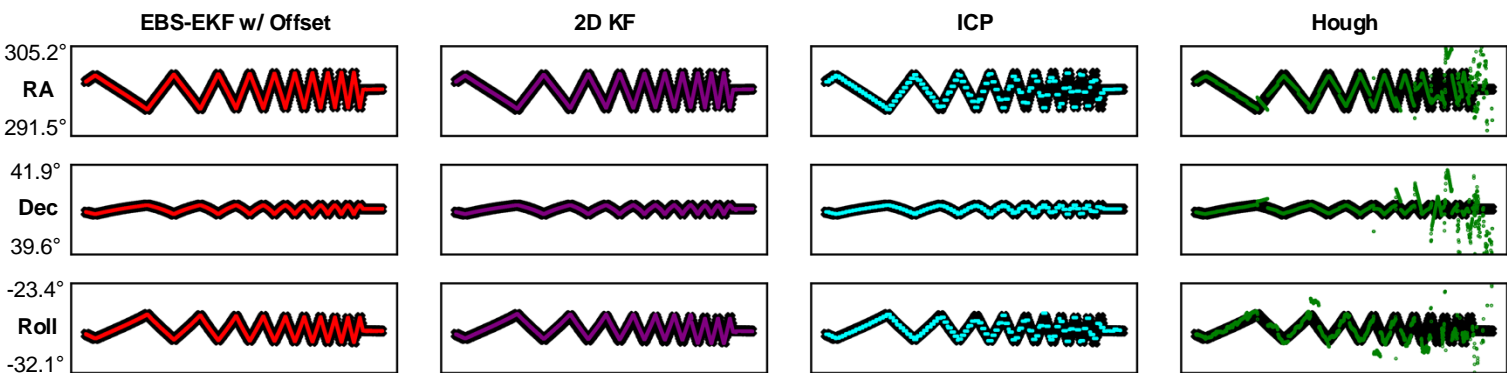

Across Difference

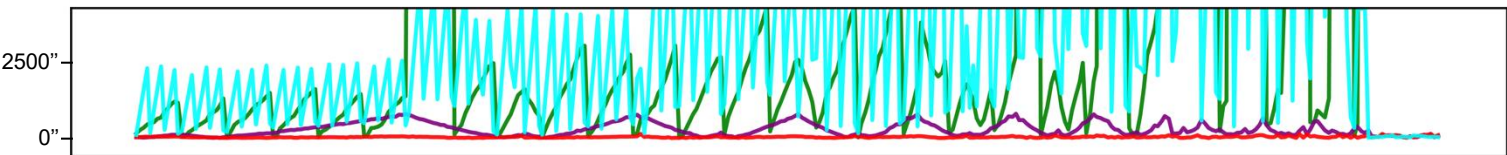

About Difference

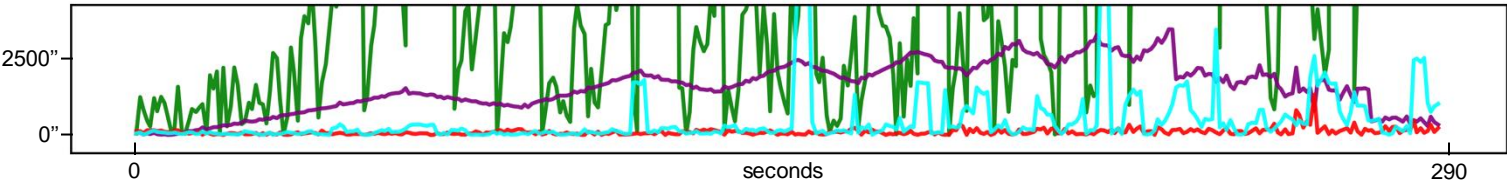

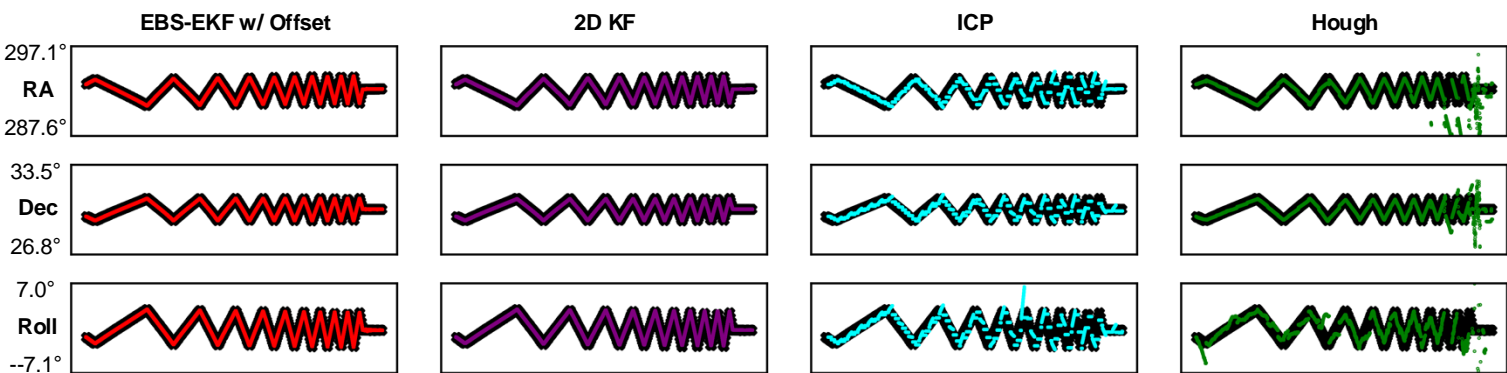

Across Difference

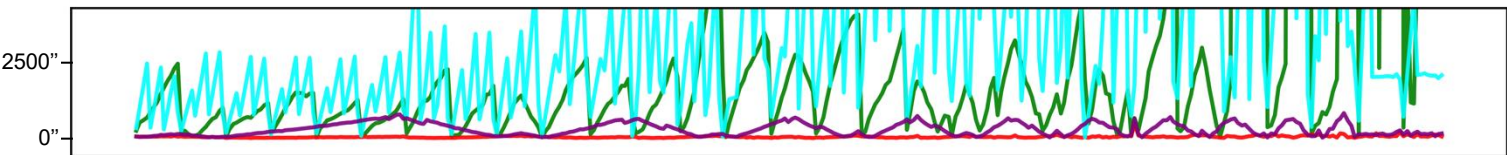

About Difference

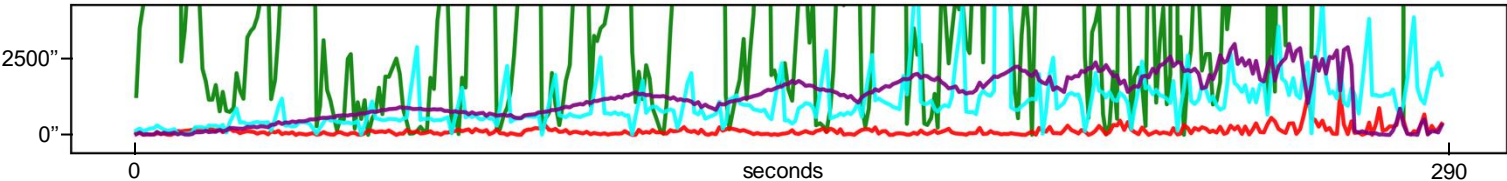

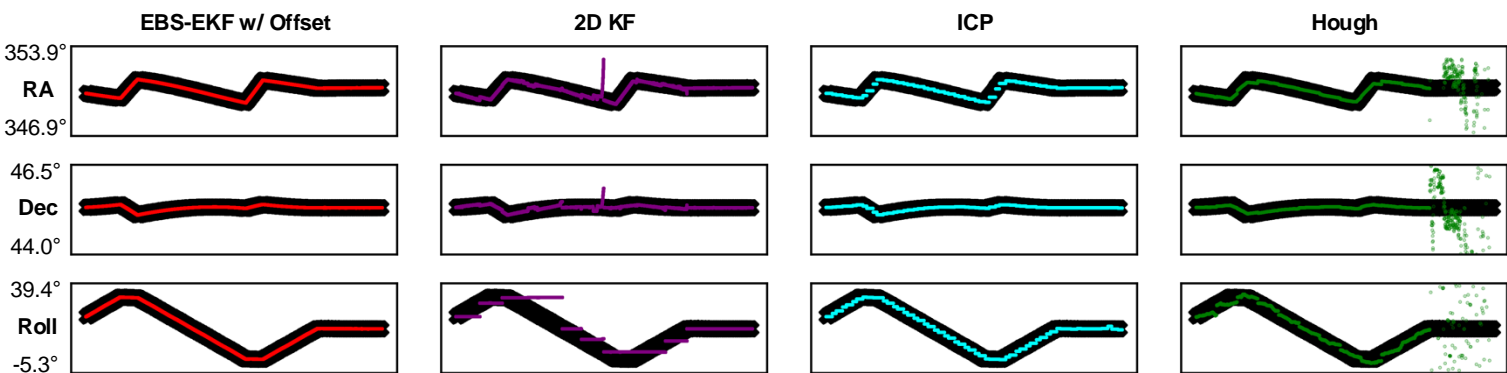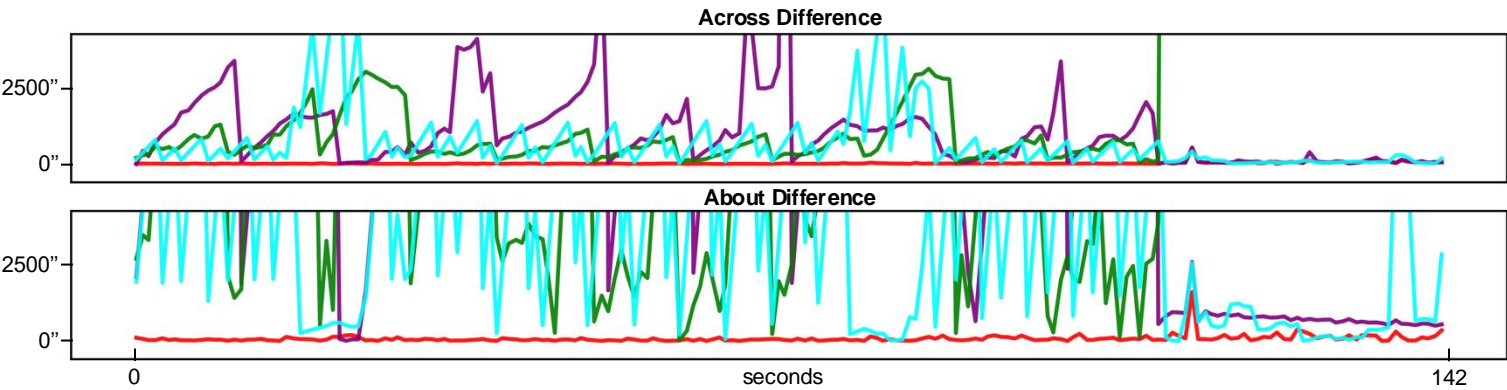

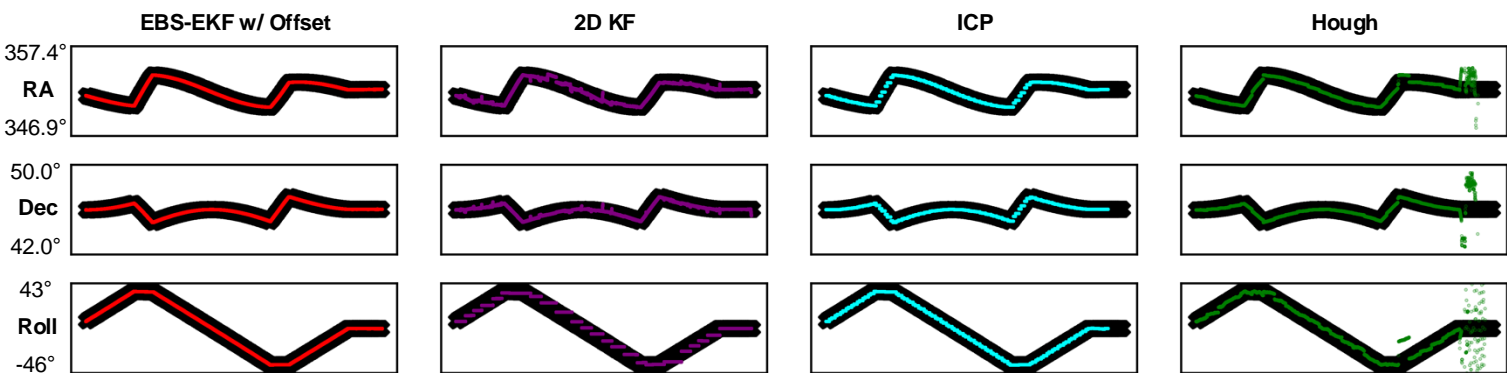

Across Difference

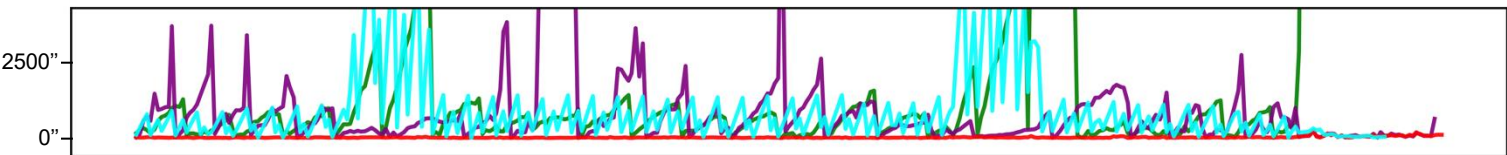

About Difference

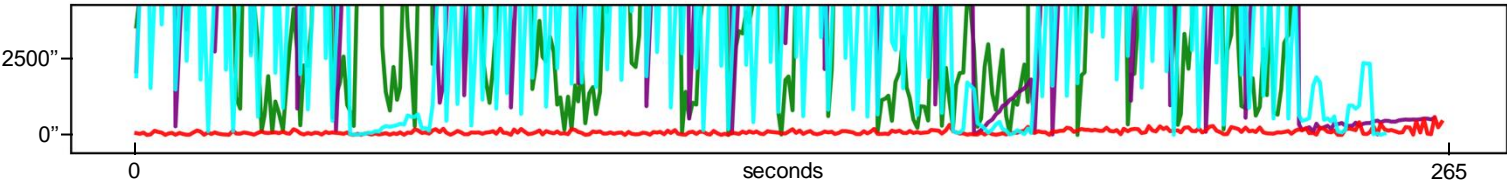

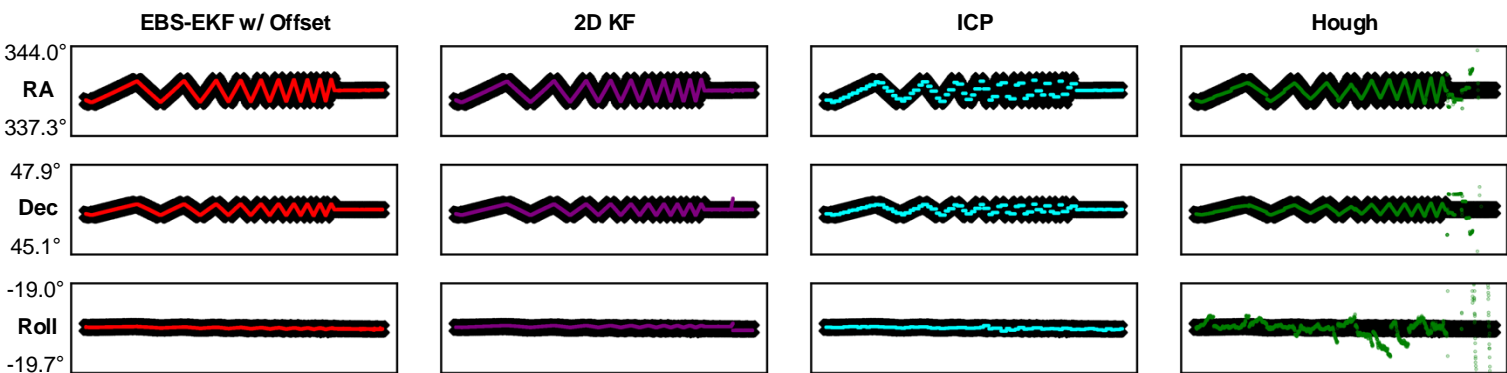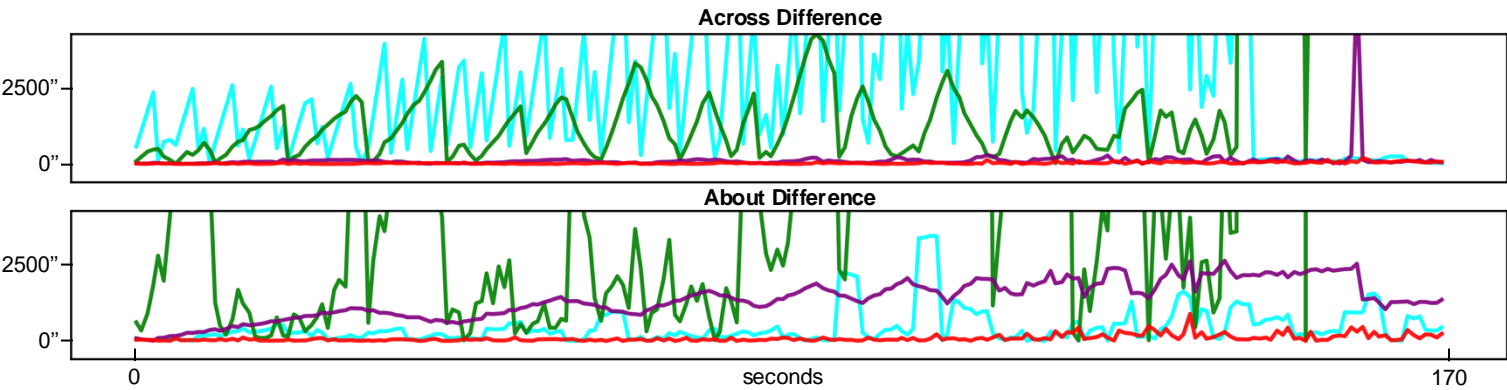



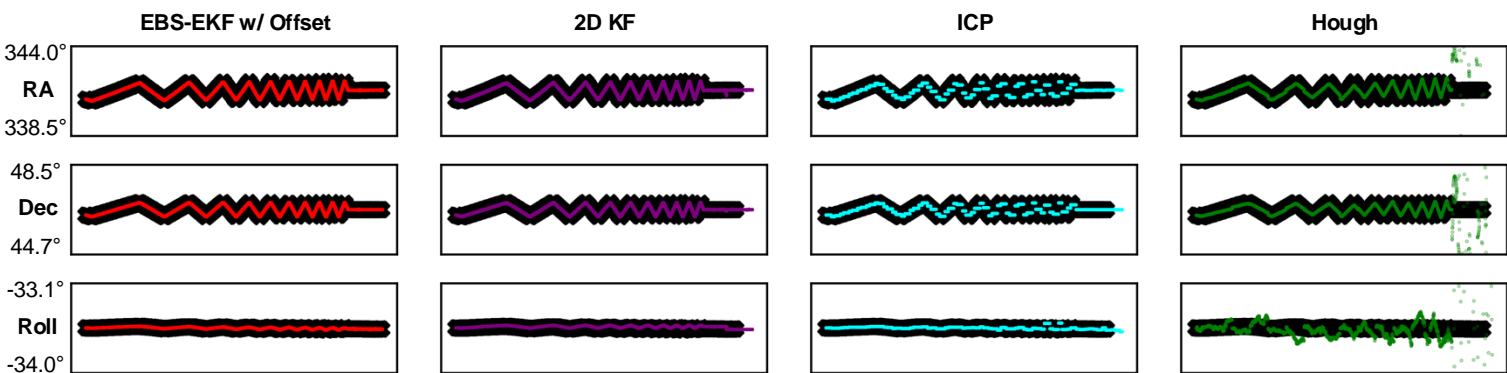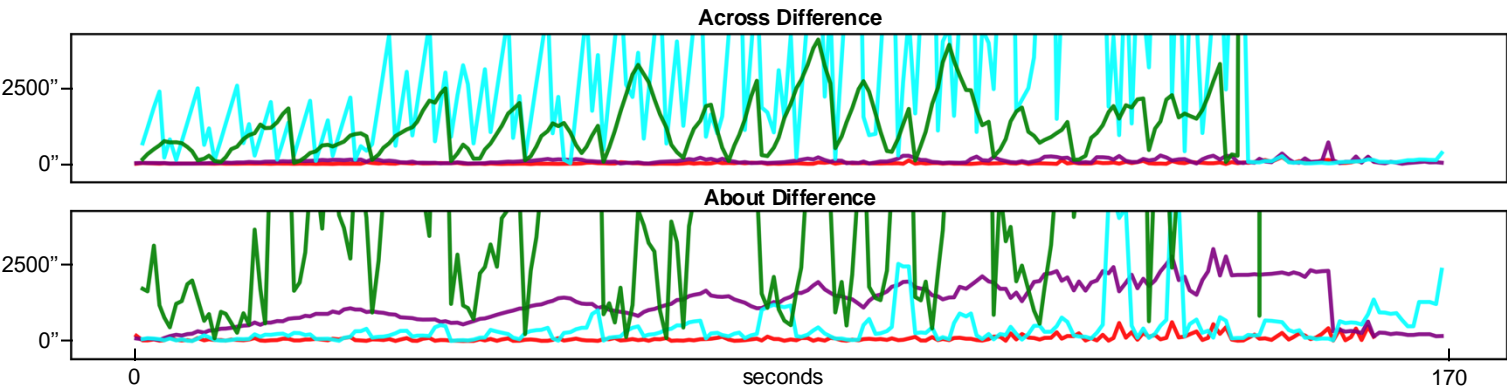



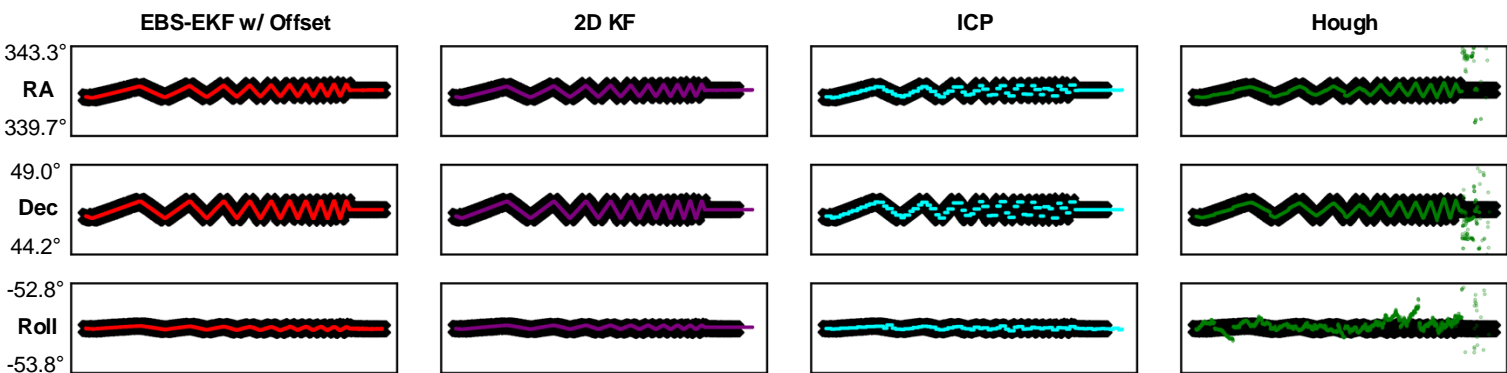

Across Difference

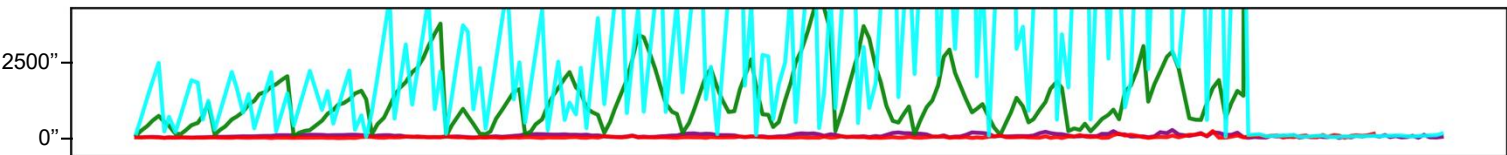

About Difference

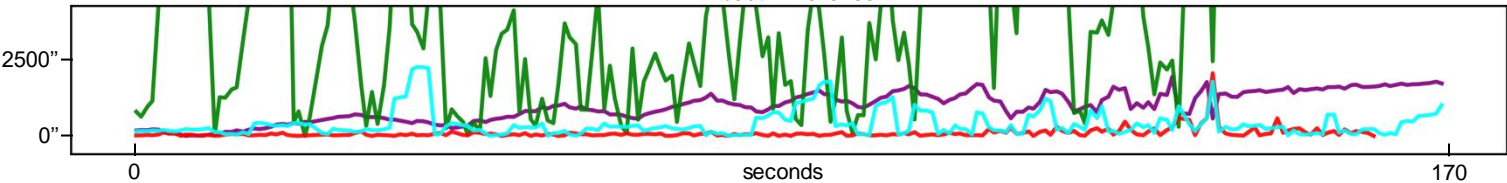

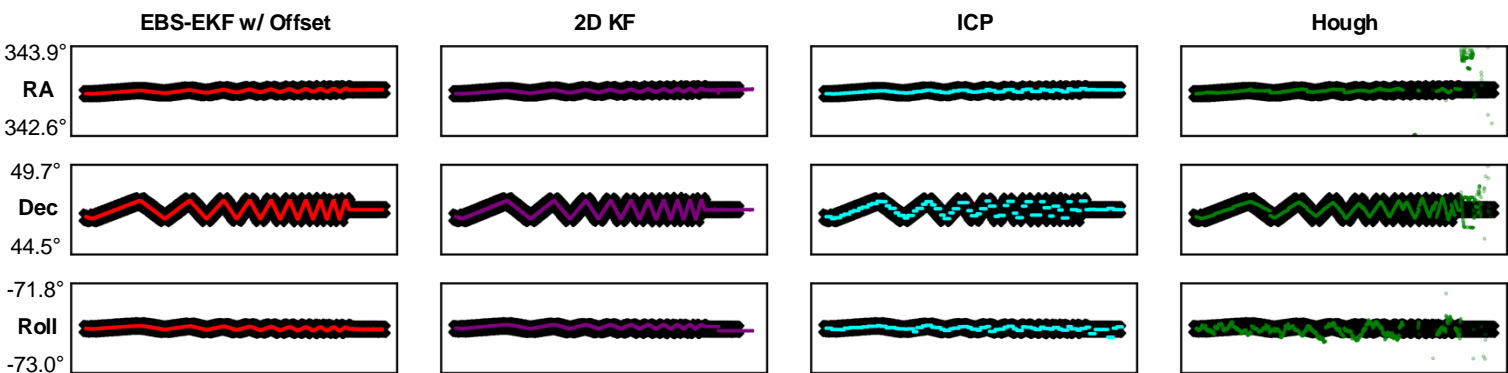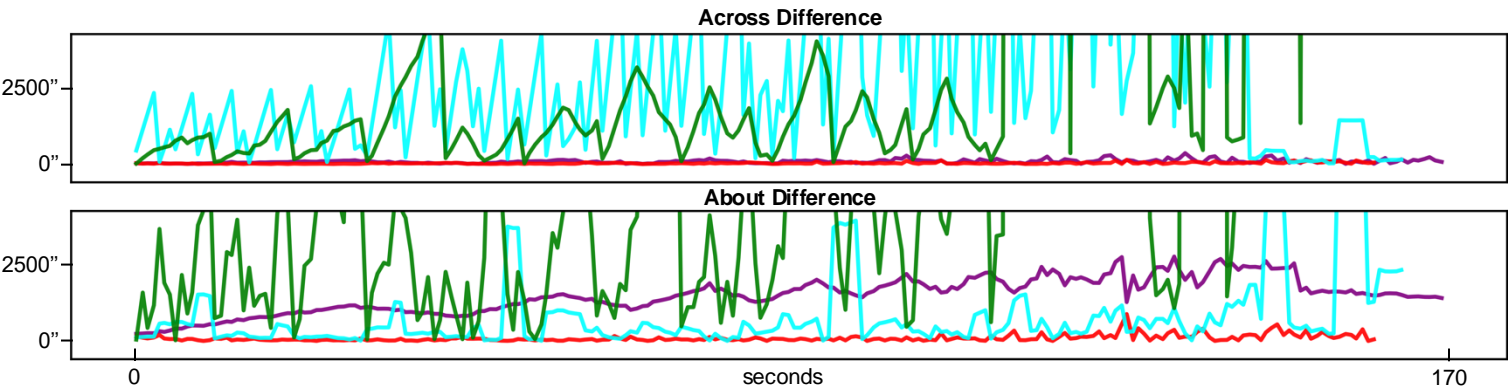

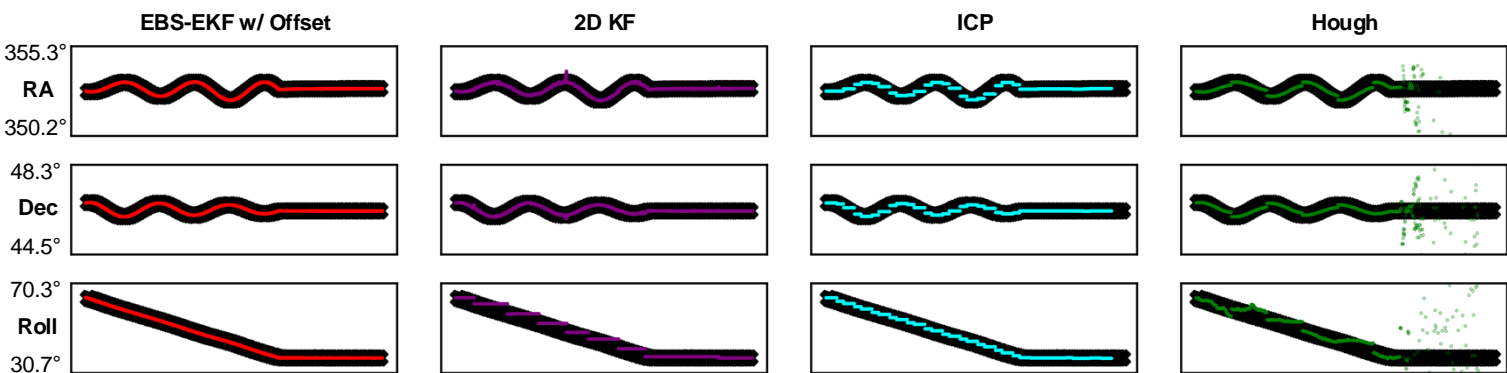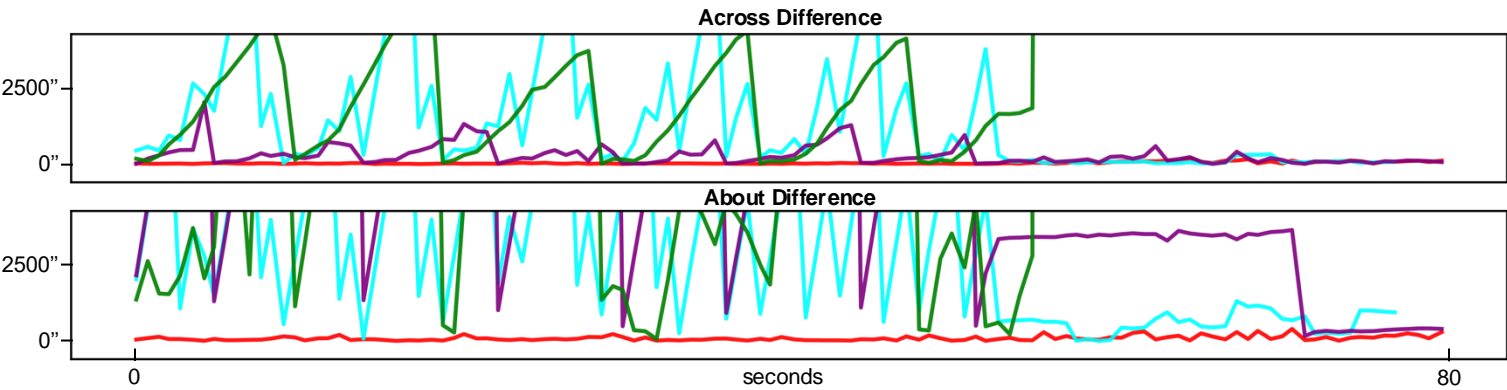

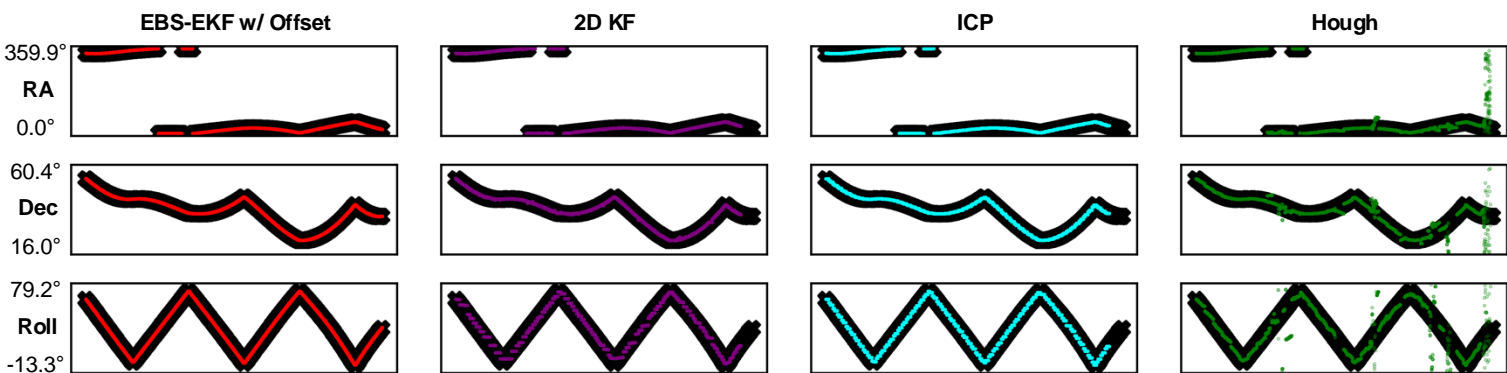

Across Difference

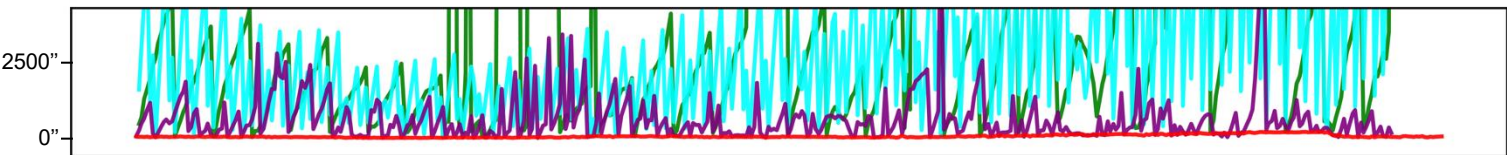

About Difference

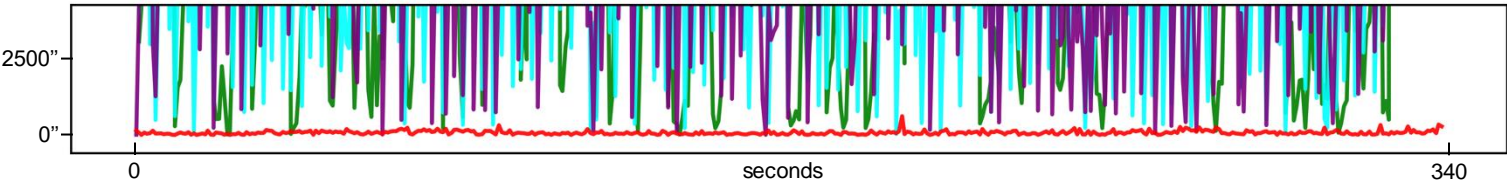

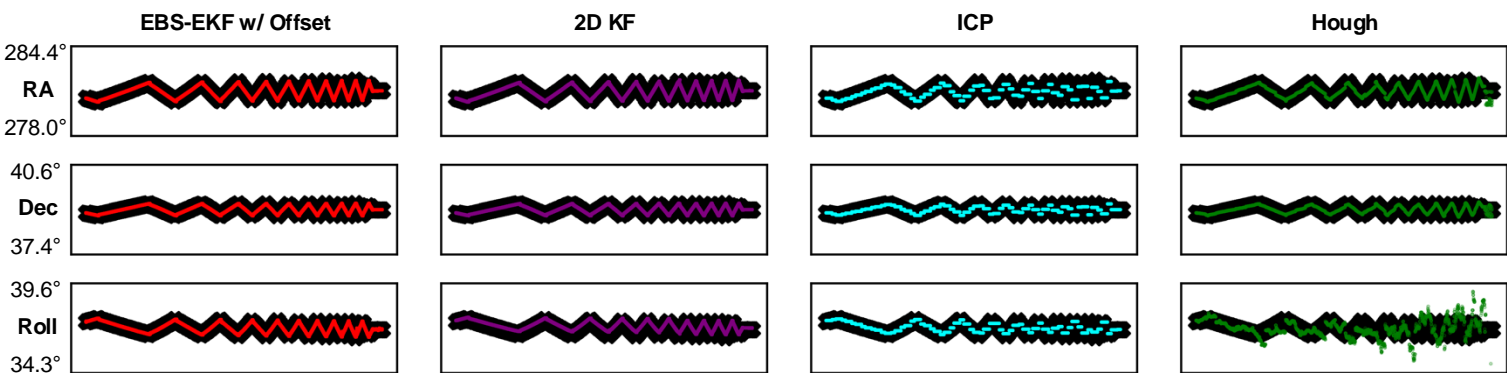

Across Difference

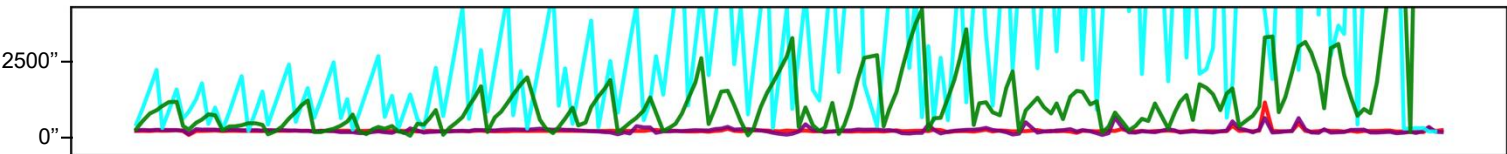

About Difference

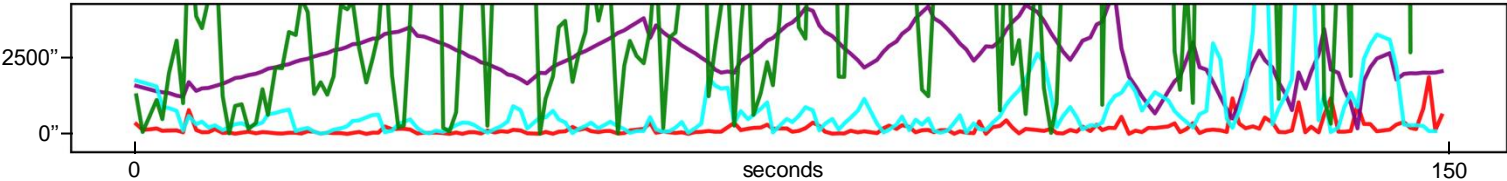

Supplement: Supplementary file 1 [file track-comparison-errors-supp.pdf]
