# Supplementary material for: EBS-EKF: Accurate and High Frequency Event-based Star Tracking
Source: arXiv:2503.20101 source file (2025-03-25)
Supplement: Supplementary file 2 [file supp_ideas.tex]

\begin{itemize}
    \item EKF math/whatever Albert wants
    \item PSF derivation (if we include it)
    \item PSF graphics (PSF functions)
    \item Possible v2e simulations if no room in paper
\end{itemize}

Current promises
\begin{itemize}
    \item PSF velocity coordinate frame conversion
    \item Additional event profile graphics
\end{itemize}
