# Supplementary material for: EBS-EKF: Accurate and High Frequency Event-based Star Tracking
Source: arXiv:2503.20101 source file (2025-03-25)
Supplement: Supplementary file 3 [file paper_todo.tex]

\begin{itemize}
    \item Prove star is Gaussian
    \item Prove space is linear instead of log or do just log
\end{itemize}
